# Supplementary material for: ReFeree: Radar-based efficient global descriptor using a Feature and Free space for Place Recognition
Source: arXiv:2403.14176 source file (2024-07-18)
Supplement: Supplementary file 1 [file additional_results.tex]

\section{Sonar Context Results}
\begin{table}[h]
\caption{Overall Performance Evaluation in single session}
\centering\resizebox{0.49\textwidth}{!}{
\begin{tabular}{c|l|ccc}
\toprule
\textbf{Sequence}         & \textbf{Approach}          & \textbf{Recall@1}    & \textbf{F1 max score} & \textbf{AUC score}   \\ \hline
\multirow{5}{*}{DCC 01}   & Radar SC                   & 0.683                & \underline{0.852}     & 0.908                \\
                          & \underline{RaPlace}        & 0.641                & 0.849                 & \underline{0.917}    \\
                          & Radar VLAD                 & 0.507                & 0.819                 & 0.885                \\
                          & Radar FFTVLAD              & \underline{0.706}    & 0.779                 & 0.874                \\
                          & \textbf{ReFeree (Ours)}    & \textbf{0.723}       & \textbf{0.861}        & \textbf{0.936}       \\ \hline
\multirow{5}{*}{KAIST 03} & \underline{Radar SC}       & 0.896                & \underline{0.966}     & \underline{0.991}    \\
                          & RaPlace                    & 0.932                & 0.938                 & 0.984                \\
                          & Radar VLAD                 & 0.833                & 0.931                 & 0.978                \\
                          & Radar FFTVLAD              & \underline{0.948}    & 0.937                 & 0.985                \\
                          & \textbf{ReFeree (Ours)}    & \textbf{0.953}       & \textbf{0.971}        & \textbf{0.992}       \\ 
\bottomrule
\end{tabular}}
\label{tab:single}
\vspace{-0.5cm}
\end{table}

\begin{table}[b]
\caption{Overall Performance Evaluation in multi session}
\centering\resizebox{0.49\textwidth}{!}{
\begin{tabular}{c|l|ccc}
\toprule
\textbf{Sequence}          & \textbf{Approach}          & \textbf{Recall@1}    & \textbf{F1 max score} & \textbf{AUC score}   \\ \hline
\multirow{5}{*}{Bellmouth} & Radar SC                   & 0.772                & 0.893                 & \underline{0.964}    \\
                           & RaPlace                    & 0.023                & 0.099                 & 0.040                \\
                           & \underline{Radar VLAD}     & \underline{0.839}    & \underline{0.909}     & 0.881                \\
                           & Radar FFTVLAD              & 0.024                & 0.127                 & 0.064                \\
                           & \textbf{ReFeree (Ours)}    & \textbf{0.978}       & \textbf{0.986}        & \textbf{0.989}       \\ \hline
\multirow{5}{*}{Maree}     & Radar SC                   & 0.634                & 0.827                 & \underline{0.902}    \\
                           & RaPlace                    & 0.351                & 0.500                 & 0.198                \\
                           & Radar VLAD                 & 0.670                & 0.779                 & 0.727                \\
                           & \underline{Radar FFTVLAD}  & \underline{0.854}    & \underline{0.897}     & 0.765                \\
                           & \textbf{ReFeree (Ours)}    & \textbf{0.995}       & \textbf{0.972}        & \textbf{0.941}       \\ \hline
\multirow{5}{*}{Hydro}     & \underline{Radar SC}       & \underline{0.954}    & \underline{0.975}     & \underline{0.970}    \\
                           & RaPlace                    & 0.799                & 0.818                 & 0.578                \\
                           & Radar VLAD                 & 0.940                & 0.911                 & 0.943                \\
                           & Radar FFTVLAD              & 0.932                & 0.899                 & 0.882                \\
                           & \textbf{ReFeree (Ours)}    & \textbf{0.989}       & \textbf{0.985}        & \textbf{0.990}       \\ 
\bottomrule
\end{tabular}}
\label{tab:oord_overall}
% \vspace{-0.4cm}
\end{table}

\begin{table}[b]
\caption{Overall Performance Evaluation in various weather}
\centering\resizebox{0.49\textwidth}{!}{
\begin{tabular}{c|l|ccc}
\toprule
\textbf{Sequence}          & \textbf{Approach}          & \textbf{Recall@1}    & \textbf{F1 max score} & \textbf{AUC score}   \\ \hline
\multirow{5}{*}{Sunny}     & Radar SC                   & 0.815                & 0.961                 & \textbf{0.994}       \\
                           & RaPlace                    & 0.816                & 0.905                 & 0.973                \\
                           & Radar VLAD                 & 0.778                & 0.899                 & 0.959                \\
                           & \underline{Radar FFTVLAD}  & \underline{0.946}    & \underline{0.973}     & 0.981                \\
                           & \textbf{ReFeree (Ours)}    & \textbf{0.966}       & \textbf{0.983}        & \textbf{0.994}       \\ \hline
\multirow{5}{*}{Overcast}  & \textbf{Radar SC}          & \textbf{0.903}       & 0.910                 & \textbf{0.970}       \\
                           & RaPlace                    & 0.830                & 0.918                 & 0.956                \\
                           & Radar VLAD                 & 0.806                & \underline{0.932}     & \underline{0.969}    \\
                           & Radar FFTVLAD              & 0.861                & 0.649                 & 0.533                \\
                           & \underline{ReFeree (Ours)} & \underline{0.880}    & \textbf{0.941}        & 0.966                \\ \hline
\multirow{5}{*}{Snowing}   & Radar SC                   & 0.520                & 0.971                 & 0.554                \\
                           & RaPlace                    & 0.848                & \underline{0.982}     & 0.996                \\
                           & \textbf{Radar VLAD}        & \underline{0.862}    & \textbf{0.992}        & \textbf{0.999}       \\
                           & Radar FFTVLAD              & 0.480                & 0.964                 & 0.994                \\
                           & \underline{ReFeree (Ours)} & \textbf{0.883}       & 0.974                 & \underline{0.998}    \\  \bottomrule

\end{tabular}}
% \vspace{-0.5cm}
\label{tab:boreas_overall}
\end{table}
